# Supplementary material for: Assessing generalisability of deep learning-based polyp detection and segmentation methods through a computer vision challenge
Source: arXiv:2202.12031 source file (2022-02-24)
Supplement: Supplementary file 1 [file supplimentaryFile1.tex]

\section{EAD2019 challenge leaderboard}
\begin{itemize}
    \item Summarize in words regarding numbers and leaderboard and methods
    \item Summary table (Sharib will do this)
    \item Link all to Suppl. Material 2 
    \begin{itemize}
        \item Leaderboard
        \item Algorithms in detail: 3-4 short paragraphs per method (till 6 top methods for detection and 6 for segmentation)
        \item Suppl. Note
        \item Executable versions if available
    \end{itemize}
\end{itemize}
